# Supplementary material for: Electrical Tuning of Fresnel Lens in Reflection
Source: arXiv:2104.05312 source file (2021-04-12)
Supplement: Supplementary file 1 [file SI_Main.pdf]

# Supporting Information for
# Electrical Tuning of Fresnel Lens in Reflection

Christopher Damgaard-Carstensen*, Martin Thomaschewski, Fei Ding, and Sergey I. Bozhevolnyi*

*Centre for Nano Optics, University of Southern Denmark, Campusvej 55, DK-5230 Odense M, Denmark*

*To whom correspondence should be addressed:
cdc@mci.sdu.dk, seib@mci.sdu.dk

## 1 Investigation of the Fabry-Perot modulator

The design of the proposed active Fresnel lens (AFL) requires an in-depth understanding of the Fabry-Perot resonators constituting the active part of our device (Figure S1a). We wish to operate the resonator around resonance to be able to tune the reflective properties. The resonance is achieved by obtaining destructive interference between the light reflected from the bottom and top gold electrode layers. Thus, it is necessary to match the reflected power from each layer and assure they are out of phase. The phase change is primarily acquired through the difference in optical path length between the two reflection channels, and it is therefore controlled by the thickness of the lithium niobate (LN) layer and the wavelength of the incident light. The reflected power is matched by appropriately selecting the thickness of the top gold layer. As mentioned in the main text, the thickness of the LN layer is $t_{LN} \simeq 300\,\mathrm{nm}$, and hence the important design parameters of the resonator are the thickness of the top gold layer and the wavelength. An amplitude map is composed by varying the top electrode thickness and incident wavelength (Figure S1b). A resonance is clearly visible at a wavelength of $\sim 840\,\mathrm{nm}$ and a thickness of $\sim 10\,\mathrm{nm}$. Our work is aimed at achieving maximum modulation efficiency, which is calculated for a DC modulation voltage of $\pm 10\,\mathrm{V}$, and shows a sharp maximum at a thickness of $t_g = 12\,\mathrm{nm}$ (Figure S1c). The maximum is relatively sharp due to the rather small shift of the resonance under the applied modulation voltage. Optimizing for highest modulation efficiency, we should use a top electrode thickness of $t_g = 12\,\mathrm{nm}$ (Figure S1d), however this poses some problems in fabrication. Experience shows that the minimum realizable film thickness, in order to achieve a homogeneous thin film, is $15\,\mathrm{nm}$ with the equipment at hand. This results in a less pronounced resonance, and thus a

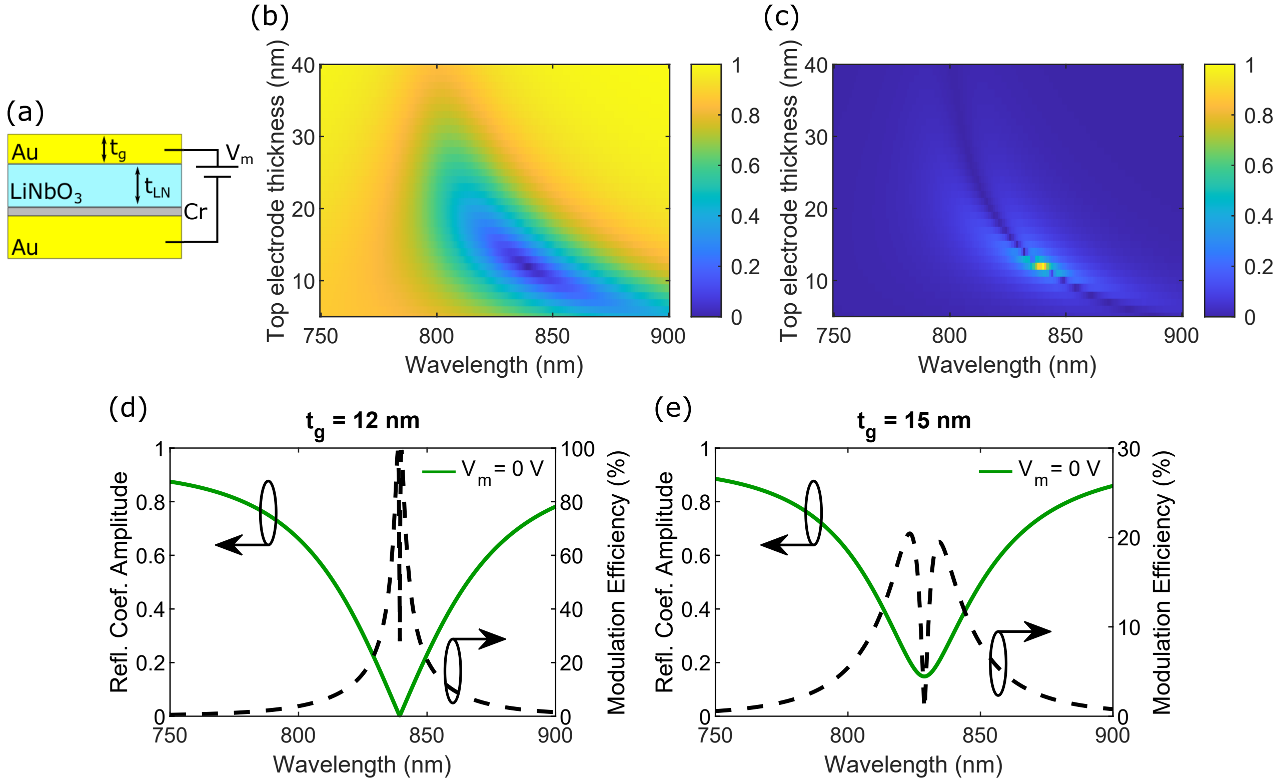


**Figure S1:** Calculated performance of a Fabry-Perot modulator. (a) Cross section sketch displaying the semi-transparent gold layer deposited on a lithium niobate thin film, adhered to a gold back-reflector by a thin chromium adhesive layer. (b) Calculated reflection coefficient amplitude as a function of thickness of the top gold layer and wavelength of the normally incident light. (c) Calculated modulation efficiency as a function of thickness of the top gold layer and wavelength for DC modulation voltages of $\pm 10$ V. (d,e) Plots of reflection coefficient amplitude (left axis) and modulation efficiency (right axis) versus wavelength for a thickness of the top gold layer of (d) $t_g = 12$ nm and (e) $t_g = 15$ nm at DC modulation voltages of $\pm 10$ V.

reduction in achievable modulation efficiency by a factor of five (Figure S1d,e), yet reliability of the homogeneity of the gold film is paramount for the experimental realization leading to the choice of using a top electrode thickness of 15 nm.

After numerical investigations, we move on to experimental characterization. Using standard electron-beam lithography and lift-off, the Fabry-Perot modulator is realized by fabricating a square with dimensions 100 µm × 100 µm, which is connected to a macroscopic electrode by a 2 µm wide stripe, in order to establish electrical connection. A scanning electron microscopy image of the square is shown in Figure S2a. Quantification of the modulator performance is carried out by comparison of the modulation efficiency determined through both simulation and experimental characterization (Figure S2b). An incident beam is limited to the square by an iris, and the modulation properties are measured when applying a modulation voltage of $\pm 10$ V (see Methods section of the main text). The measured data show a shifted resonance compared to the previously calculated data (Figure S1e and S2b), which is primarily due to variation in the thickness of the LN thin film. Based on the measured data, an adjusted thickness of 323 nm is determined by matching the spectral position of the resonance. The

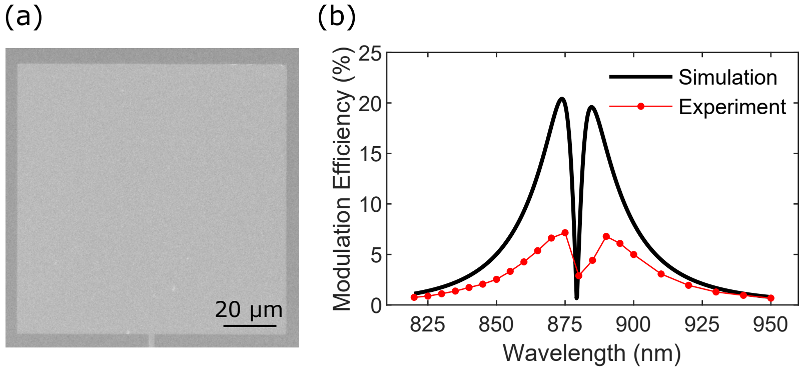


**Figure S2:** Experimental characterization of a Fabry-Perot modulator. (a) Scanning electron microscopy image of a gold square of 100 µm × 100 µm used for characterization of the modulator. (b) Calculated and measured modulation efficiency of the modulator as a function of wavelength for a modulation voltage of ±10 V. Error bars are in the order of data point sizes. The thickness of the lithium niobate thin film for calculation of the modulation efficiency is adjusted to match the resonance of the measured data. This results in an adjusted thickness of 323 nm.

obtained results show good correspondence between the shapes of the curves, although the measured modulation efficiency is a factor of two lower than the calculated one. We believe these additional losses are due to various factors, including absorption in the titanium adhesion layer or inhomogeneity in the semitransparent gold thin film, yet we achieve significantly higher modulation efficiencies than those obtained with a similar structure using electro-optic polymers [1].

## 2 Determination of design wavelength

After having determined the optimal thickness of the top gold electrode, we wish to determine the design wavelength leading to maximum modulation of the intensity in the focal spot. To do so, wavelength dependence of the focusing efficiency is simulated for DC modulation voltages of 0 and ±10 V for a lens design that is updated for each iteration of the wavelength (Figure S3a). A significant increase in focusing efficiency from ∼3 to ∼20 % is present in the investigated wavelength range, and the largest difference in focusing efficiency, due to the applied modulation voltage, occurs at the part of steepest slope. Comparing to Figure S1e, the maximum focusing efficiency is achieved far from the Fabry-Perot resonance of the resonator. The reason for this is found in the phase response (Figure S3c). Focusing from a Fresnel lens in reflection can be achieved in two ways: By eliminating reflected light from each alternating zone, or by assuring the reflected light from alternating zones is out of phase. We design the AFL using the first approach, thus alternating reflective and absorbing zones, because this allows for modulation of the focal spot intensity by tuning the reflectivity of the absorbing zones. However, this approach limits the maximum achievable focusing efficiency, as much of the incident light is absorbed. The phase response of the Fabry-Perot resonator shows that at the wavelength of 950 nm, corresponding to maximum focusing efficiency, the incident light experiences a phase shift of ∼ 180° from the resonator compared to areas without top gold electrodes, thus causing the AFL to

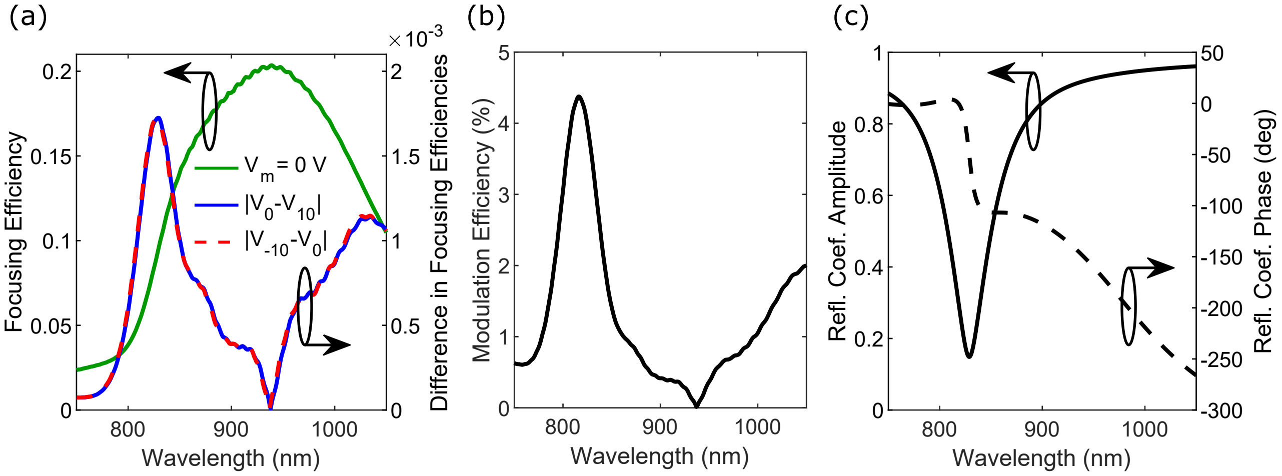


**Figure S3:** Determining the optimal Fresnel lens design wavelength. (a,b) The investigated lens dimensions are updated for each iteration of the incident wavelength. (a) Calculated focusing efficiency (left axis) as a function of wavelength for no modulation voltage, and variation in focusing efficiency (right axis) when applying DC modulation voltages of ±10 V. (b) Calculated modulation of the focusing efficiency as a function of wavelength, when applying DC modulation voltages of ±10 V. (c) Investigation of the evolution of reflection coefficient amplitude and reflected phase with wavelength for the Fabry-Perot resonator.

focus using the second approach leading to increased focusing efficiency. Investigation of the graphs (Figure S3a,b), show, however, that the maximum in focusing efficiency comes with a minimum in modulation efficiency, thus resulting in the choice of a design wavelength of 815 nm, which points to the largest modulation efficiency at the cost of lower focusing efficiency.

## 3 Electro-optical characterization of the AFL

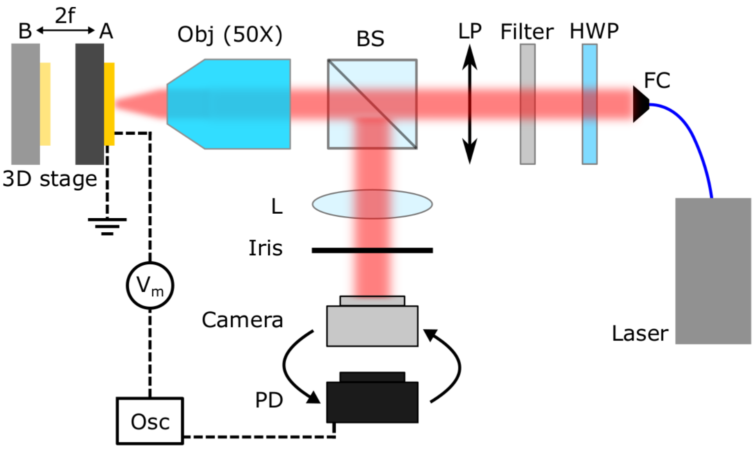


**Figure S4:** Schematic of the optical setup used for characterization of the AFL. The optical path is indicated by red while the electrical wiring is indicated by black dashed lines. A and B represent two planes, separated by a distance of twice the focal length, where the incident light and reflected light from the AFL produce a focused spot, respectively. FC: Fiber-coupling, HWP: Half-wave plate, LP: Linear polarizer, L: Lens, BS: Beam splitter, Obj: Objective, PD: Photodetector, Osc: Oscilloscope, $V_m$: Modulation voltage source.

The fabricated AFL is characterized using a setup similar to those previously used for characterizing focusing metasurfaces (Figure S4) [2, 3]. An incident low-power continuous wave laser beam is focused to a spot on flat unstructured gold (plane A in Figure S4) by a long working distance 50X objective. The focusing effect of the AFL is visualized by shifting the sample a distance of $2f$ to the plane where the reflected light is tightly focused (plane B in Figure S4). Reflected light is separated from the incident light by a beam splitter and viewed on a camera or photodetector depending on which characteristic is under investigation (see Methods section of the main text).

# 4 Comparison of electrically tunable thin lenses

| | Ref. [4] | Ref. [5] | Ref. [6] | **Our work** |
|---|---|---|---|---|
| Focusing efficiency | 65 % | 2 % (BSt) | 0.06 % | **15 %** |
| Modulation efficiency | - | - | 33 % | **1.5 %** |
| Wavelength range (nm) | 445 – 630 | 1500 – 1530 | 550 – 650 | **800 – 900** |
| Modulation voltage (V) | ±50 | ±6 | +3 | **±10** |
| Electrical bandwidth | - | - | < 25 Hz* | **4 MHz** |
| Possibility for reconfiguration | Dynamic control of focal length | Dynamic beam steering or focusing | - | **-** |
| Ease of fabrication | FIB | Multi-step lithography | Multi-step lithography | **One-step lithography** |
| Material platform | Multilayer graphene | ITO | $WS_2$/ graphene | **LN** |

*Estimation from rise/fall times

**Table S1:** Comparison of recently published works on electrically tunable thin lenses with our work, comparing several key characteristics. Abbreviations are: BSt: Beam steering, FIB: Focused ion beam milling, ITO: Indium tin oxide, $WS_2$: Tungsten disulfide, LN: Lithium niobate

# References


[1] J. Zhang, Y. Kosugi, A. Otomo, Y.-L. Ho, J.-J. Delaunay, Y. Nakano, and T. Tanemura, "Electrical tuning of metal-insulator-metal metasurface with electro-optic polymer," *Applied Physics Letters*, vol. 113, p. 231102, Dec. 2018.

[2] A. Pors, M. G. Nielsen, R. L. Eriksen, and S. I. Bozhevolnyi, "Broadband focusing flat mirrors based on plasmonic gradient metasurfaces," *Nano Letters*, vol. 13, pp. 829–834, Jan. 2013.

[3] S. Boroviks, R. A. Deshpande, N. A. Mortensen, and S. I. Bozhevolnyi, "Multifunctional metamirror: Polarization splitting and focusing," *ACS Photonics*, vol. 5, pp. 1648–1653, Oct. 2017.

[4] S. Park, G. Lee, B. Park, Y. Seo, C. bin Park, Y. T. Chun, C. Joo, J. Rho, J. M. Kim, J. Hone, and S. C. Jun, "Electrically focus-tuneable ultrathin lens for high-resolution square subpixels," *Light: Science & Applications*, vol. 9, June 2020.

[5] G. K. Shirmanesh, R. Sokhoyan, P. C. Wu, and H. A. Atwater, "Electro-optically tunable multi-functional metasurfaces," *ACS Nano*, vol. 14, pp. 6912–6920, Apr. 2020.

[6] J. van de Groep, J.-H. Song, U. Celano, Q. Li, P. G. Kik, and M. L. Brongersma, "Exciton resonance tuning of an atomically thin lens," *Nature Photonics*, vol. 14, pp. 426–430, Apr. 2020.
